# Supplementary material for: Scalable Video Object Segmentation with Identification Mechanism
Source: arXiv:2203.11442 source file (2024-05-28)
Supplement: Supplementary file 1 [file id_bank_appendix.tex]

\begin{figure}[h!]
\begin{center}

\begin{subfigure}[t]{.24\linewidth}
			\centering
			\includegraphics[width=0.8\linewidth]{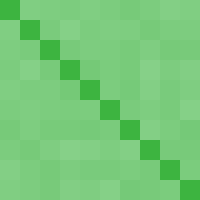}
			\caption{$M=10$}\label{fig:id_bank_10}
\end{subfigure}
\begin{subfigure}[t]{.24\linewidth}
			\centering
			\includegraphics[width=0.8\linewidth]{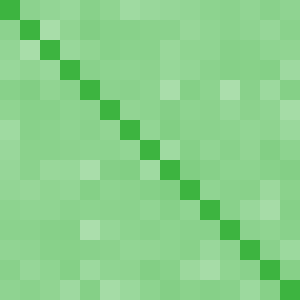}
			\caption{$M=15$}\label{fig:id_bank_15}
\end{subfigure}
\begin{subfigure}[t]{.24\linewidth}
			\centering
			\includegraphics[width=0.8\linewidth]{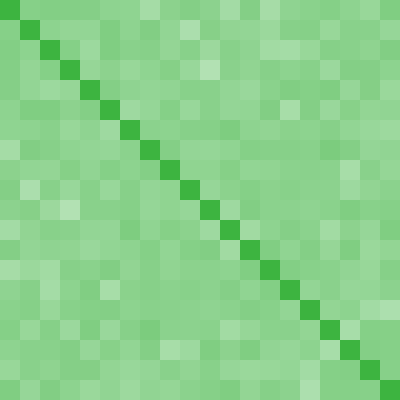}
			\caption{$M=20$}\label{fig:id_bank_20}
\end{subfigure}
\begin{subfigure}[t]{.24\linewidth}
			\centering
			\includegraphics[width=0.8\linewidth]{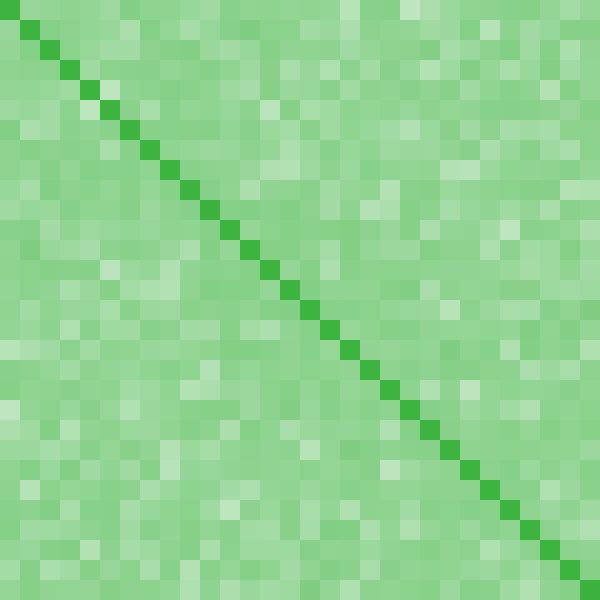}
			\caption{$M=30$}\label{fig:id_bank_30}
\end{subfigure}

\end{center}

\caption{\textbf{Visualization of the cosine similarity between every two of $n_{id}$ identification vectors in the identity bank}. The results are visualized in the form of a symmetric matrix measuring $n_{id}\times n_{id}$. Diagonal values in this matrix are set to 1. Darker colors in the matrix indicate higher levels of similarity. We observe stable and equitable similarities when $n_{id}=10$. However, when $n_{id}$ increases, the matrix becomes less uniform, leading to a greater degree of instability in the similarities.}\label{fig:id_bank}
\end{figure}
