# Supplementary material for: Scalable Video Object Segmentation with Identification Mechanism
Source: arXiv:2203.11442 source file (2024-05-28)
Supplement: Supplementary file 2 [file occlusion_appendix.tex]

\begin{wrapfigure}[19]{r}{0.45\textwidth}
    \centering\vspace{-10mm}
    \includegraphics[width=0.93\linewidth]{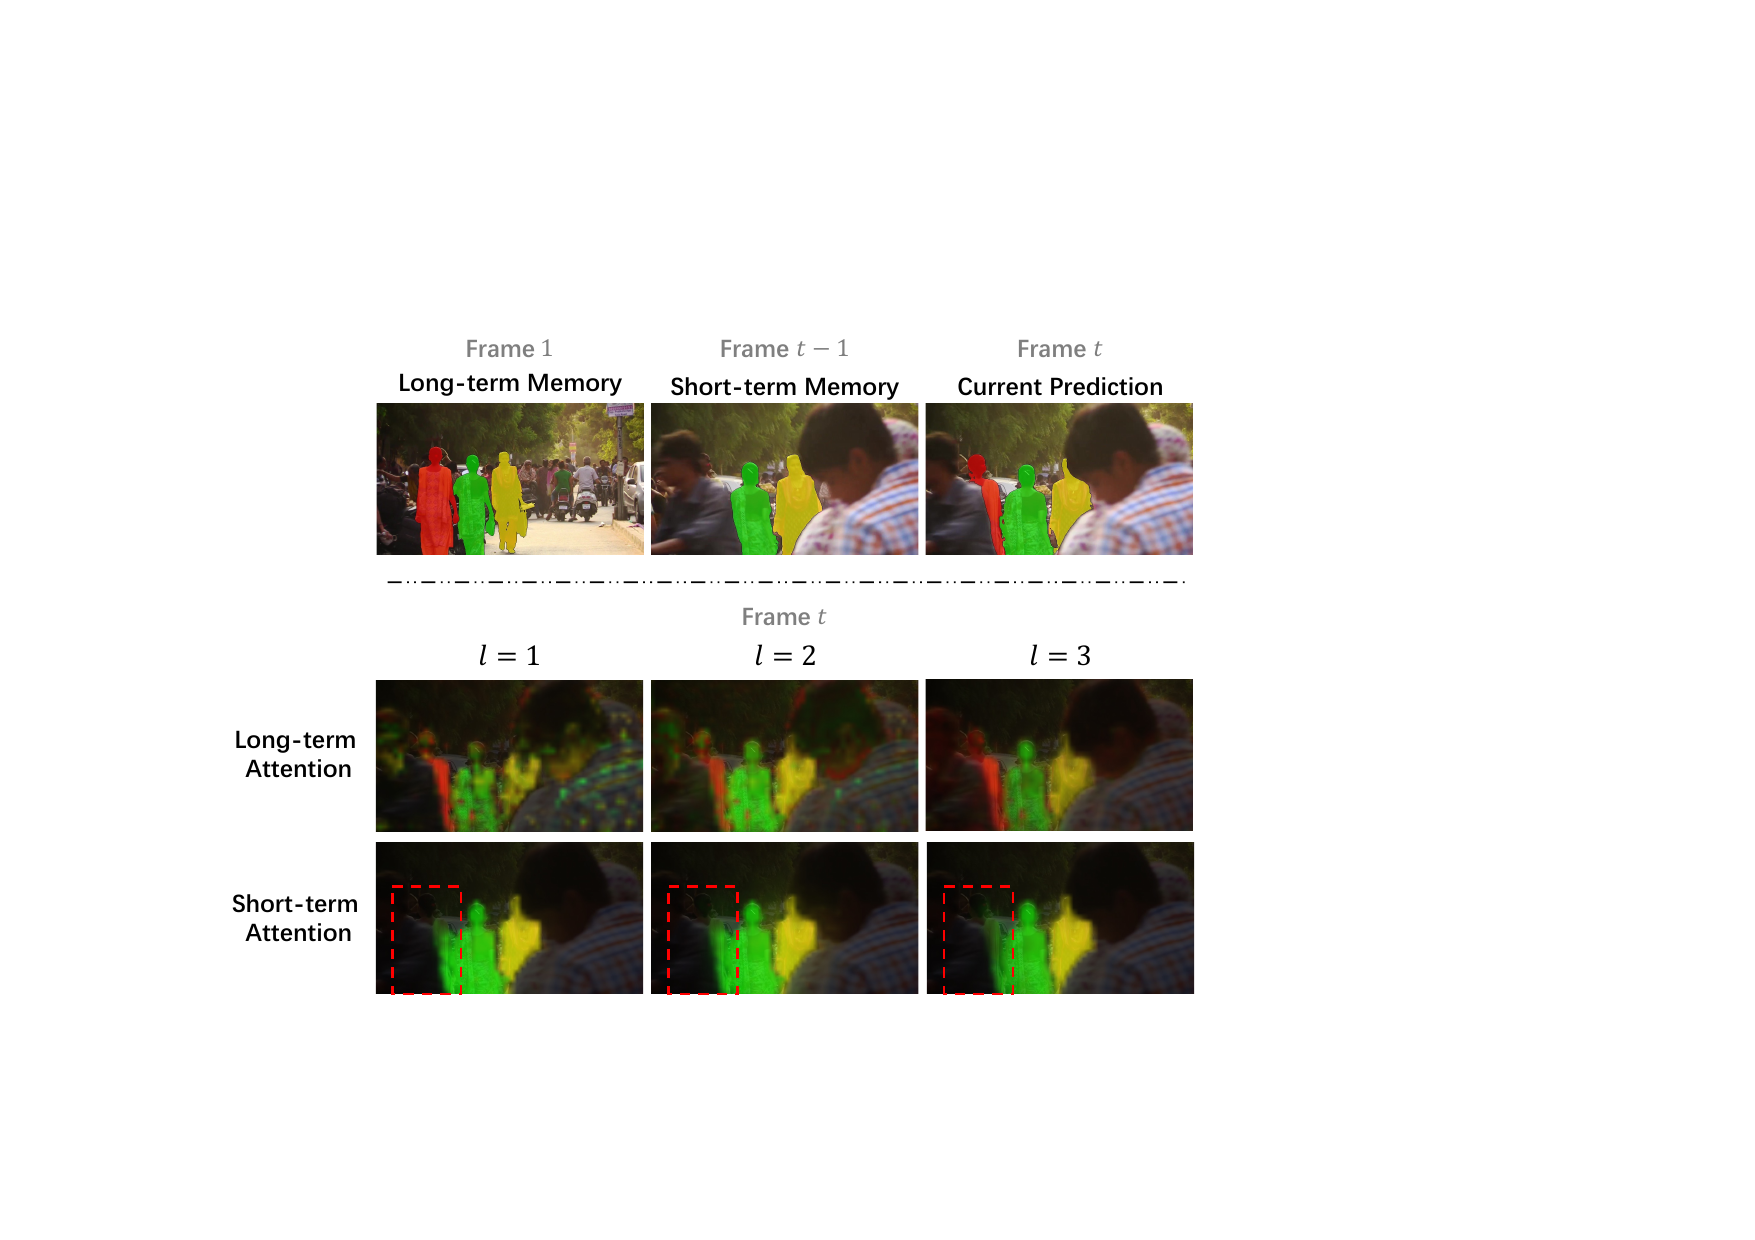}

    \caption{Visualization of long-term and short-term attention maps of our approaches on DAVIS 2017~\cite{davis2017}. The video has three similar people, marked in different colors, and the red person is occluded in frame $t-1$. For visualization, we propagate the colored multi-object masks in long-term or short-term memory to the current frame regarding the corresponding attention maps. The brighter the color, the stronger the attention. 
    % Here, the red person is occluded in Frame $t-1$; thus, the short-term attention fails to match the person. However, long-term attention generates an accurate attention map with a clean background in the last layer, $l=3$, resulting in a correct prediction.
    }
    \label{fig:occlusion}

\end{wrapfigure}
